# Supplementary material for: Teaching Cameras to Feel: Estimating Tactile Physical Properties of Surfaces From Images
Source: arXiv:2004.14487 source file (2021-09-20)
Supplement: Supplementary file 1 [file Appendix.tex]

\subsection{Appendix A}

\begin{table}[]
\centering
\caption{\textbf{Tactile descriptions} Each of the fifteen tactile dimensions measured by the Toccare device are defined below.}
\resizebox{\textwidth}{!}{
\begin{tabular}{|c|c|l|}
\hline
    & Tactile Dimension       & \multicolumn{1}{c|}{Description}                                                                                                                                        \\ \hline
fRS & Sliding Resistance      & \begin{tabular}[c]{@{}l@{}}The perceived effort required to initiate sliding on a surface,\\ ranging from low grip to high grip.\end{tabular}                           \\ \hline
fST & Tactile Stiction        & \begin{tabular}[c]{@{}l@{}}The perceived effort required to continue sliding over a surface, \\ranging from slippery to resistive.\end{tabular}                         \\ \hline
uCO & Microtexture Coarseness & \begin{tabular}[c]{@{}l@{}}The perceived spacing of small ($<$1mm spacing) features,\\ ranging from fine to coarse.\end{tabular}                                          \\ \hline
uRO & Microtexture Roughness  & \begin{tabular}[c]{@{}l@{}}The intensity of small ($<$1mm) features that \\creates the perception of roughness, ranging from smooth to rough.\end{tabular}                \\ \hline
mRG & Macrotexture Regularity & \begin{tabular}[c]{@{}l@{}}The perceived uniformity of large ($>$1mm spacing) features, ranging\\ from random to regular.\end{tabular}                                    \\ \hline
mCO & Macrotexture Coarseness & \begin{tabular}[c]{@{}l@{}}The perceived spacing of large ($>$1mm spacing) features, ranging\\ from fine to coarse.\end{tabular}                                          \\ \hline
mTX & Macrotexture            & \begin{tabular}[c]{@{}l@{}}The intensity of large ($>$1mm) features that creates the perception\\ of texture, ranging from smooth to textured.\end{tabular}               \\ \hline
tCO & Thermal Cooling         & \begin{tabular}[c]{@{}l@{}}The initial rate that a surface draws heat from the fingertip,\\ ranging from warm to cool.\end{tabular}                                     \\ \hline
tPR & Thermal Persistence     & \begin{tabular}[c]{@{}l@{}}The extent to which a surface continues to draw heat from \\ the fingertip, ranging from transient cooling to sustained cooling.\end{tabular} \\ \hline
cCM & Tactile Compliance      & \begin{tabular}[c]{@{}l@{}}The degree to which a surface deforms under pressure, \\ ranging from rigid to compliant.\end{tabular}                                        \\ \hline
cDF & Local Deformation       & \begin{tabular}[c]{@{}l@{}}The degree to which the surface wraps around the fingertip\\ when being deformed, ranging from flat to high wrap.\end{tabular}               \\ \hline
cDP & Damping                 & \begin{tabular}[c]{@{}l@{}}The speed with which a surface returns to its original \\shape after being deformed, ranging from springy to damped.\end{tabular}            \\ \hline
cRX & Relaxation              & \begin{tabular}[c]{@{}l@{}}The degree to which a surface stops pushing back after being\\ deformed, ranging from maintaining force to relaxing.\end{tabular}            \\ \hline
cYD & Yielding                & \begin{tabular}[c]{@{}l@{}}The degree to which a surface remains deformed after being pressed, \\ranging from recovering shape to remaining deformed.\end{tabular}      \\ \hline
aTK & Adhesive Tack           & \begin{tabular}[c]{@{}l@{}}The perceived effort required to break contact with a surface,\\ ranging from no adhesion to sticky.\end{tabular}                            \\ \hline
\end{tabular}
}
\label{tab:tactile_dim_descriptions}
\end{table}

\subsection{Appendix B}

\subsubsection{Additional Training Details}
TODO
